# Supplementary material for: Mixture Content Selection for Diverse Sequence Generation
Source: arXiv:1909.01953 source file (2019-09-04)
Supplement: Supplementary file 1 [file appendix-attn_text_fig.tex]

\begin{figure}
\begin{center}
\begin{small}
\begin{tabularx}{\linewidth}{p{\linewidth-1em}}
\toprule

\textbf{Passage-Answer}: formed in november 1990 by the equal merger of sky television and british satellite broadcasting , \ul{bskyb} became the uk 's largest digital subscription television company . \\
\textbf{Target}: who is the uk 's largest digital subscription television company ? \\
\midrule

\textcolor{blue}{\textbf{Focus 1}}:
formed in november 1990 by the equal \textcolor{blue}{merger} of \textcolor{blue}{sky television} and \textcolor{blue}{british satellite broadcasting} , \ul{bskyb} became the \textcolor{blue}{uk 's} largest digital subscription television \textcolor{blue}{company} . \\
$\Rightarrow$ who was the merger of sky television and british satellite broadcasting ? \\
\midrule

\textcolor{green}{\textbf{Focus 2}}:
formed in november 1990 by the equal merger of sky television and british satellite broadcasting , \ul{bskyb} became the \textcolor{green}{uk} 's largest digital subscription television company . \\
$\Rightarrow$ what team won the uk ? \\
\midrule

\textcolor{red}{\textbf{Focus 3}}:
formed in november 1990 by the equal merger of sky television and british satellite broadcasting , \ul{bskyb} \textcolor{red}{became} the \textcolor{red}{uk 's largest digital subscription television company} . \\
$\Rightarrow$ who became the uk 's largest digital subscription television company ? \\

\bottomrule
\end{tabularx}
\end{small}
\end{center}
\caption{
    Sample questions produced by our method from given passage-answer pair (answer is underlined).
    By selecting different tokens to focus (colored), our method generates diverse questions.
}
\label{fig:attn_text}
\end{figure}
