# Supplementary material for: Mixture Content Selection for Diverse Sequence Generation
Source: arXiv:1909.01953 source file (2019-09-04)
Supplement: Supplementary file 2 [file 05-results-t-sm-human.tex]

\begin{table}[!h]
    \resizebox{\columnwidth}{!}{
    \begin{tabular}{l||ccc||ccc}
        \hline
         & \multicolumn{3}{c||}{Diversity (\%)} & \multicolumn{3}{c}{Accuracy (\%)} \\
        \hline
        \multicolumn{1}{c||}{Baselines} & Win & Lose & Tie & Win & Lose & Tie \\
        vs. 3-D. Beam & \textbf{50.4} & 40.9 & 8.7 & \textbf{46.2} & 38.5 & 15.3 \\
        vs. 3-T. Sampling & \textbf{48.7} & 42.0 & 9.3 & \textbf{50.3} & 41.2 & 8.5 \\
        vs. 3-M. Decoder & \textbf{49.7} & 39.6 & 10.7 & \textbf{46.5} & 37.5 & 16.0 \\
        \hline
    \end{tabular}
    }
    \caption{
    Human evaluation on CNN-DM abstract summarization.
    }
    \label{table:human_sm}
\end{table}
