# Supplementary material for: Mixture Content Selection for Diverse Sequence Generation
Source: arXiv:1909.01953 source file (2019-09-04)
Supplement: Supplementary file 4 [file appendix-t1.tex]

\begin{table*}[!t]
\centering
\resizebox{\linewidth}{!}{%
    \begin{threeparttable}
        \begin{tabular}{l||c|c|c|c}
            \hline
            \multicolumn{1}{c||}{\multirow{2}{*}{Method}}
                & BLEU-4  & Oracle BLEU-4 & Average BLEU-4  & Pairwise BLEU-4 \\
            \multicolumn{1}{c||}{}
                & (Top-1 Acc.) $\Uparrow$ & (Target Coverage) $\Uparrow$ & (Average Acc.) $\Uparrow$ & (Diversity) $\Downarrow$ \\
            \hline
            NQG++ \cite{Zhou2017} & 13.27 & - & - & -\\
            \hline
            \multicolumn{5}{c}{Search-based Methods} \\
            \hline
            NQG++ \& Beam-3 & 13.590 & 16.848 & 12.977 & 67.277 \\
            NQG++ \& Beam-5 & 13.526 & 18.809 & 12.724 & 74.674 \\
            NQG++ \& Diverse Beam-3 & 13.696 & 16.989 & 13.195 & 68.018 \\
            NQG++ \& Diverse Beam-5 & 13.379 & 18.298 & 12.567 & 74.795 \\
            NQG++ \& Truncated Sampling-3 & 11.890 & 15.447 & 10.312 & 37.372 \\
            NQG++ \& Truncated Sampling-5 & 11.530 & 17.651 & 10.312 & 45.990 \\
            \hline
            \multicolumn{5}{c}{Mixture of Experts + Greedy Decoding} \\
            \hline
            NQG++ \& 3-Mixture Decoder & 14.720 & 19.324 & \textbf{13.571} & 51.360 \\
            NQG++ \& 5-Mixture Decoder & 15.166 & 21.965 & 13.267 & 58.727 \\
            NQG++ \& 3-Mixture Selector (ours) & \textbf{15.874} & 20.437 & 12.799 & 47.493 \\
            NQG++ \& 5-Mixture Selector (ours) & 15.672 & \textbf{22.451} & 12.427 & 59.815 \\
            NQG++ \& 3-Mixture Selector + Regularizer (ours) & 14.8 & 20 & 12 & \textbf{34} \\
            \hline
        \end{tabular}
    \end{threeparttable}}
\caption{
    Comparison of diverse generation methods for question generation on SQuAD dataset.
    The score of NQG++ (top row) is from \citet{Zhou2017},
    and the rest are from our experiments using NQG++ as generator.
    Each number in the method name indicates the number of generated questions for each passage-answer pair.
    Best scores are bolded.
}
\label{table:1_full}
\end{table*}
