# Supplementary material for: Mixture Content Selection for Diverse Sequence Generation
Source: arXiv:1909.01953 source file (2019-09-04)
Supplement: Supplementary file 5 [file appendix-t2.tex]

\begin{table*}[!h]
    \centering
    \resizebox{\linewidth}{!}{%
    \begin{tabular}{l||c|c|c|c|c|c}
        \hline
        \multicolumn{1}{c||}{\multirow{2}{*}{Method}}
            & R-1 & R-2 & R-L & Oracle R-2 & Average R-2 & Pairwise R-2 \\
        \multicolumn{1}{c||}{}
            & \multicolumn{3}{c|}{(Top-1 Acc.) $\Uparrow$} & (Target Coverage) $\Uparrow$ & (Average Acc.) $\Uparrow$ & (Diversity) $\Downarrow$ \\
        \hline
        PG \cite{See2017} & 39.53 & 17.28 & 36.38 & - & - & - \\
        \hline
        \multicolumn{7}{c}{Search-based Methods} \\
        \hline
        PG \& Beam-3 & 38.189 & 16.533 & 35.576 & 18.509 & 16.538 & 85.598 \\
        PG \& Beam-5 & 38.216 & 16.634 & 35.401 & 19.442 & 16.623 & 84.765 \\
        PG \& Diverse Beam-3 & 38.324 & 16.667 & 35.457 & 18.722 & 16.707 & 85.496 \\
        PG \& Diverse Beam-5 & 38.302 & 16.632 & 35.357 & 19.659 & 16.620 & 84.043 \\
        PG \& Truncated Sampling-3 & 35.744 & 12.914 & 33.015 & 17.068 & 11.880 & 17.306 \\
        PG \& Truncated Sampling-5 & 35.872 & 13.049 & 33.121 & 19.161 & 11.658 & \textbf{16.720} \\
        \hline
        \multicolumn{7}{c}{Mixture of Experts + Greedy Decoding} \\
        \hline
        PG \& 3-Mixture Decoder & 36.665 & 15.854 & 33.917 & 21.214 & 15.646 & 43.168 \\
        PG \& 5-Mixture Decoder & 37.027 & 16.104 & 34.264 & 21.801 & 15.784 & 67.196 \\
        PG \& 3-Mixture Selector (ours) & 40.324 & 17.930 & 37.273 & 21.316 & \textbf{17.499} & 51.092 \\
        PG \& 5-Mixture Selector (ours) & \textbf{40.689} & \textbf{18.309} & \textbf{37.535} & \textbf{22.511} & 17.099 & 47.280 \\
        \hline
    \end{tabular}
    }
    \caption{
        Comparison of diverse generation methods for abstract summarization on CNN-DM dataset.
        R stands for ROUGE \cite{Lin2004}.
        The score of Pointer Generator (PG; top row) is from \citet{See2017},
        and the rest are from our experiments using PG as generator.
        Each number in the method name indicates the number of generated summaries for each source document.
        Best scores are bolded.
        }
    \label{table:2_full}
\end{table*}
